# Supplementary material for: Better Understanding, Better Fixes? A Study of Hallucination in LLM-based Automated Program Repair
Source: arXiv:2609.04909 source file (2026-09-28)
Supplement: Supplementary file 1 [file appendix.tex]

\section{Prompts}
\label{app:prompts}

\subsection{Prompt for Triggering Test Identification}
\label{app:prompt-triggering-test}

\begin{lstlisting}[style=promptstyle]
You are an expert software debugging and program analysis assistant.

Task:
Given:
1. Source code: The complete functions where an error occurs. If multiple functions are buggy, all will be provided.
2. Testcases: All relevant testcases.

Your job is to:
- Determine which testcase methods actually expose the bug.
- Produce the minimal correct fix.
- Return the result in the required JSON format only.

Your Workflow
1. Analyze all buggy functions carefully.
2. Evaluate each testcase method by tracing execution across all relevant functions.
3. Identify only the testcase methods that truly trigger the bug.
4. Provide the full corrected implementation of all input functions. fixed_code must include every function from the input, in the same order, regardless of whether it was modified by you.

Rules:
- The defect may be caused by a single function or by multiple functions working together.
- If multiple functions collectively cause the issue, you must fix all of them.
- Output every testcase method that actually triggers the bug.
- Do not include testcase methods that do not trigger the bug.
- For each triggering testcase, it must fail on the buggy version but pass on your fixed version.
- Preserve original functionality as much as possible.
- The fix must be minimal but correct.

Example Output Format:
{
  "trigger_method": [
    "full_trigger_method_path1",
    "full_trigger_method_path2",
    ...
  ],
  "fixed_code": [
    "full fixed_function1 as a JSON string", 
    "full fixed_function2 as a JSON string",
    ...
  ]
}

Hard constraints:
- Output ONLY the JSON object; NO explanations or comments inside/outside the JSON object.
- Use double quotes for all keys/strings. No trailing commas.
\end{lstlisting}

\newpage
\subsection{Prompt for Line Coverage Prediction}
\label{app:prompt-line-coverage}

\begin{lstlisting}[style=promptstyle]
You are an expert software debugging and program analysis assistant. 

Task:
Given:
1. Source code: The complete functions where an error occurs. If multiple functions are buggy, all will be provided.
2. Trigger testcases: All trigger testcases.

Your job is to:
- Predict buggy coverage: union of executed lines per function across all triggers.
- Fix the bug: modify all necessary functions.
- Predict fixed coverage: union of executed lines per function across all triggers.

Your Workflow
1. Analyze all buggy functions: Analyze the execution paths of the buggy functions under all trigger functions, and identify which lines of each buggy function are covered (union across triggers).
2. Provide the fix: Output the entire corrected implementation of the functions (not a diff). If the bug spans multiple functions, provide fixed implementations for all of them. fixed_code must include every input function, in the same order, even if unchanged.
3. Analyze all fixed functions:
Analyze the execution paths of the fixed functions under all trigger functions, and identify which lines are covered (union across triggers).

Rules:
Output line numbers ONLY for lines executed by at least one trigger (union).
For each function, number every physical line starting from 1. Numbering resets per function (function_1 starts at 1, function_2 starts at 1, etc.).Count lines exactly as shown, including: blank lines, comment lines, lines containing only { or }, lines containing only whitespace. 
Original functionality must remain unchanged. If any external dependencies are missing, you must ask for them--never invent them.
Make the fix minimal but correct.

Example Output Format:
{
  "function_1": {
    "buggy": [1, 4, 5, 6],
    "fixed": [1, 3, 4, 7]
  },
  "function_2": {
    "buggy": [2, 3],
    "fixed": [2, 3]
  },
  "fixed_code": [
    "fixed function_1",
    "fixed function_2"
  ]
}

Hard constraints:
- Output ONLY the JSON object; NO explanations or comments inside/outside the JSON object.
- Use double quotes for all keys/strings. No trailing commas.
\end{lstlisting}

\newpage
\subsection{Prompt for Additional Test Generation}
\label{app:prompt-additional-testcase}

\begin{lstlisting}[style=promptstyle]
You are an expert software debugging and program analysis assistant. 

Task:
Given:
1. Source code: The complete functions where an error occurs. If multiple functions are buggy, all will be provided.
2. Trigger testcases: All trigger testcases.

Your job is to:
- Fix the bug: modify all necessary functions.
Multiple functions may jointly cause the bug; fix all of them.
- Generate additional trigger testcase(s): create the minimal number of new testcases such that
   - Every generated testcase MUST fail on the original buggy version (i.e., does NOT pass).
   - Every generated testcase MUST pass on your fixed version generated previously.
   - The generated testcases should maximize coverage of different behaviors/branches in both buggy code and generated fixed code while using the minimal number of testcases, and the explored branches should be as different as possible from those covered by the provided trigger testcases.
   - Each testcase must have a corresponding path end with .java. The path must be one of the exact file paths of the provided trigger testcases.

Your Workflow
1. Analyze all buggy functions: Understand the expected behavior from code + triggers. Identify root cause and any multi-function interactions.
2. Provide the fix: Output the entire corrected implementation of the functions (not a diff). If the bug spans multiple functions, provide fixed implementations for all of them. fixed_code must include every input function, in the same order, even if unchanged.
3. Generate additional trigger testcases: Produce the MINIMAL number of new testcases. Each new testcase must FAIL on buggy code and PASS on fixed code. Aim to cover new branches/behaviors not already exercised by the provided trigger testcases.

Rules:
- Original intended functionality must remain unchanged; fix must be minimal but correct.
- If any external dependencies are missing, you MUST ask for them--never invent them.
- Testcases must be runnable in the same environment/style as the provided triggers.
- Additional testcases should be minimal in number but maximize behavioral diversity.
- Ensure determinism and avoid flaky timing/randomness unless the original triggers already use it.
- For each function, number every physical line starting from 1. Numbering resets per function (function_1 starts at 1, function_2 starts at 1, etc.). Count lines exactly as shown, including: blank lines, comment lines, lines containing only { or }, and lines containing only whitespace.

Example Output Format:
{
  "fixed_code": [
    "fixed function_1",
    "fixed function_2"
  ],
  "additional_testcases": [
    {
      "path": "testcase_1_path",
      "testcase": "testcase_1_code"
    },
    {
      "path": "testcase_2_path",
      "testcase": "testcase_2_code"
    }
  ]
}

Hard constraints:
- Output ONLY the JSON object; NO explanations or comments inside/outside the JSON object.
- Use double quotes for all keys/strings. No trailing commas.
\end{lstlisting}


\newpage
\subsection{Prompt for the Baseline Repair Setting}
\label{app:prompt-baseline}

\begin{lstlisting}[style=promptstyle]
You are a senior software engineer.

Task:
Given:
The complete functions where an error occurs. If multiple functions are buggy, all will be provided.

Your job is to:
- Produce the minimal correct fix.
- Return the result in the required JSON format only.


Your Workflow
1. Analyze all buggy function(s) carefully.
2. Provide the full corrected implementation of all input functions. fixed_code must include every function from the input, in the same order, regardless of whether it was modified by you.

Rules:
- The defect may be caused by a single function or by multiple functions working together.
- If multiple functions collectively cause the issue, you must fix all of them.
- Preserve original functionality as much as possible.
- The fix must be minimal but correct.

Output Format:
{
  "fixed_code": [
    "full fixed_function1 as a JSON string", 
    "full fixed_function2 as a JSON string",
    ...
  ]
}

Hard constraints:
- Output ONLY the JSON object; NO explanations or comments inside/outside the JSON object.
- Use double quotes for all keys/strings. No trailing commas. 

\end{lstlisting}
